# Supplementary material for: Discontinuous rigidity transition associated with shear jamming in granular simulations
Source: arXiv:2301.12179 ancillary file (2023-01-28)
Supplement: Supplementary file 1 [file Discontinuous_rigidity_SM.pdf]

# Supplemental Material of "Discontinuous rigidity transition associated with shear jamming in granular simulations"

Here we provide addition results and details regarding the simulations in "Discontinuous rigidity transition associated with shear jamming in granular simulations"

## CONTENTS


I. Details of Discrete Element Method (DEM) simulation 1

II. Pebble game algorithm 2

III. Identifying rattlers 4

IV. $P_\infty$ for finite rate shear with $\mu = 1.0$ 4

V. Rigidity transition for system with $\mu = 0.1$ 5
A. Finite rate shear 5
B. Quasi-static shear with $\mu = 0.1$. 5

VI. Determining mobilized contacts 6

VII. Over-constrained networks and floppy modes in frictional and frictionless shear 6

References 7


## I. DETAILS OF DISCRETE ELEMENT METHOD (DEM) SIMULATION

Friction is implemented in the simulations as follows. Two particles are in contact when there is a finite overlap $\delta$ between them. This will result in a repulsive force between the particles which is modeled using a harmonic spring. One can also model it using a non-linear spring, then the interaction is Hertzian. Along with the repulsive spring, there is also a damping term that depends on the component of the relative velocity along the vector connecting the centers of the two springs. Therefore the repulsive force acting between two particles $i$ and $j$ is

$$\mathbf{F}_N = k_n \delta \mathbf{n}_{ij} - m_{eff} \eta_n \mathbf{v}_n \tag{1}$$

where $k_n$ is the stiffness of the repulsive spring, $\eta_n$ is the co-efficient of damping, $\delta$ is $\frac{\sigma_i+\sigma_j}{2} - |\mathbf{r}_{ij}|$, $\mathbf{n}_{ij}$ is the unit vector connecting the centers of the two disks in contact and $\mathbf{v}_n$ is the component of the relative velocity of the two disks along $\mathbf{n}_{ij}$, $\mathbf{v}_n = (\mathbf{v}_j - \mathbf{v}_i) \cdot \mathbf{n}_{ij} \mathbf{n}_{ij}$. $m_{eff} = m_i m_j/(m_i + m_j)$ is the effective mass. The friction that acts between the particles is modeled using a tangential spring with a stiffness co-efficient $k_t$. In addition to the spring, there is also a damping term that depends on the relative tangential velocity just like the normal component. This contribution to the contact force is

$$\mathbf{F}_t = k_t \mathbf{\Delta s} - m_{eff} \eta_t \mathbf{v}_t \tag{2}$$

where $\mathbf{\Delta s}$ is the tangential displacement acquired during the existence of the contact and $\mathbf{v}_t$ is the tangential relative velocity. The tangential relative velocity is given by

$$\mathbf{v}_t = (\mathbf{v}_r - \mathbf{v}_n) - (R_i \Omega_i - R_j \Omega_j) \times \mathbf{n}_{ij} \tag{3}$$

where

$$\mathbf{v}_r = \mathbf{v}_i - \mathbf{v}_j \tag{4}$$

and $\Omega_i$ is the angular velocity of particle $i$. The tangential displacement is then calculated as

$$\mathbf{\Delta s}_t = \int_{t_0}^{t} \mathbf{v}_t dt. \tag{5}$$

When computing $\mathbf{\Delta s}_t$ we have to take care of the tumbling rotation of the pair in contact which changes the tangential plane, this is done by removing any component of the tangential displacement along $\mathbf{n}_{ij}$ and rescaling to preserve the magnitude [1]. Therefore the entire force acting between two particles is,

$$\mathbf{F}_{ij} = (k_n \delta \mathbf{n}_{ij} - m_{eff}\eta_n \mathbf{v}_n) - (k_t \mathbf{\Delta s}_t + m_{eff}\eta_t \mathbf{v}_t). \tag{6}$$

With this force, one writes the equations of motion for the system

$$m_i \frac{d^2\mathbf{r}_i}{dt} = \sum_j \mathbf{F}_{ij} - \eta \mathbf{v}_i \tag{7}$$

$$I_i \frac{d\Omega_i}{dt} = \sum_j \mathbf{F}^t_{ij} R_i - \eta \Omega_i \tag{8}$$

where the $\eta$ term represents a global damping term, for both translational and rotational motion. This helps the system reach force balance faster and can be thought of as arising from the friction of the granular material with the bottom plate of the experiment. The simulations are done using LAMMPS [2]. The simulation units we use are: length $[L] = \sigma$ , energy $[E] = k_n\sigma^2/2 = \epsilon$, mass $[M] = m$, and time $[T] = \sigma\sqrt{m/\epsilon}$.

| | $k_n$ | $K_t$ | $\Delta\gamma$ | $\eta_n$ | $\eta_t$ | $\mu$ | $\eta$ | $dt$ | $\rho_{disk}$ | $\sigma_2/\sigma_1$ | $\phi$ | $N$ |
|---|---|---|---|---|---|---|---|---|---|---|---|---|
| I | 2. | 2. | $10^{-4}$ | 3. | $\frac{1}{2}\eta_n$ | 1. | $\frac{m}{0.35}$ | 0.002 | 1. | 1.4 | 0.81 | 16384 |
| II | 2. | 2. | $10^{-3}$ | 3. | $\frac{1}{2}\eta_n$ | 1. | $\frac{m}{0.35}$ | 0.002 | 1. | 1.4 | 0.81 | 2000 |
| III | 1. | 1. | $10^{-4}$ | 0.1 | $\frac{1}{2}\eta_n$ | 0.1 | 10m | 0.002 | 1. | 1.4 | 0.83 | 4096 |
| IV | 1. | 1. | $10^{-3}$ | 0.1 | $\frac{1}{2}\eta_n$ | 0.1 | 0.1m | 0.002 | 1. | 1.4 | 0.83 | 4096 |

TABLE I. Values used in the simulations. The first column represents the different sets of simulations: I is for the $\mu = 1.0$ finite rate simulations described in the main draft. II is for the $\mu = 1.0$ quasi-static simulations described in the main draft. III is for the finite rate shear simulations for $\mu = 0.1$ described in this SI. IV is for the quasi-static shear simulations with $\mu = 0.1$ described in SM.

## II. PEBBLE GAME ALGORITHM

As mentioned in the main text, the pebble game algorithm is an algorithm to check if a given 2D graph is rigid or not. If a graph is rigid, then the nodes of the graph cannot be moved without changing the length of the edges. Any such displacement of vertices such that the length of the edges does not change is called a floppy mode. In the context of jamming, the graph we analyze for rigidity is the contact network. The particle centers become the vertices of the graph, and each contact is represented by an edge in this graph. According to Laman's Theorem [3] a graph in $2D$ with $N$ sites and $2N - 3$ edges is minimally rigid iff there exist no subgraph with $n$ sites and more than $2n - 3$ edges. A subgraph that violates this condition is called over-constrained. The pebble game is an algorithm to check if this condition is valid for a given graph. The pebble game starts with each vertex having $k = 2$ pebbles indicating the degrees of freedom each vertex has and we try to cover every edge with a pebble indicating a degree of freedom lost in the system due to the edge following the rules of the pebble game which we describe below. The number of free pebbles (the ones that remain on the vertices) after the pebble game indicates the number of floppy modes the system has. We cannot constrain $l = 3$ degrees of freedom as these are two global translations and a rotation. The original $(k = 2, l = 3)$ pebble game algorithm by [4] was extended to general $(k, l)$ pebble game by Lee and Streinu [5] which we described below. We use $(k = 2, l = 2)$ pebble game for frictionless contact network and $(k = 3, l = 2)$ for frictional contact network. Since we use periodic boundary condition $l = 2$ as the global rotation is not floppy mode.

- **Initialization**

  1. The pebble game starts with all vertices having $k$ pebbles each and all edges are uncovered. Any site cannot have more than $k$ pebbles at any time.

- **Assigning pebbles to bonds**

  1. Consider an edge $E$ that connects vertices $a$ and $b$.

2. The rule for covering an edge is that the total number pebbles at its vertices is atleast $l + 1$. Then use a pebble from $a$ or $b$ to cover $E$. The edge is now directed from $a(b)$ to $b(a)$ if a pebble of $a(b)$ is used (this pebble is now used to cover $E$ and is not free).

- **Allowed pebble moves.**

1. If the sites $a$ and $b$ together do not have $l + 1$ free pebbles, then it means that pebbles are used to cover other edges connected to $a$ or $b$.
2. We can free a pebble at either sites by searching along the directed edges. Consider an edge $E'$ that is connects $a$ and $a'$ and a pebble of $a$ is used to cover $E'$. If $a'$ has a free pebble, then that pebble can be used to cover $E'$ and the pebble that was covering $E'$ can be freed. In doing so the direction of $E'$ is reversed. If $a'$ does not have a free pebble, then one can repeat the same process on the edges directed away from $a'$ and try to free a pebble and so on. The process is repeated on all the edges directed away from $a$. Similarly at $b$. So that at the end of the directed search we have $l + 1$ free pebbles for covering $E$. Note that we can always free $l$ pebbles because they are associated with global degrees of freedom.

- **Identifying independent and redundant bonds**

1. All edges covered by pebbles are marked independent.
2. If we can't cover $E$ after the pebble search, then $E$ is marked a redundant bond and all the sites visited in the failed directed search are over-constrained.
3. This process is repeated till all edges are either marked independent or redundant.

- **Rigid cluster decomposition.**

1. We will assign a label to each independent edge such that all independent edges belonging to the same rigid cluster will have the same label.
2. Consider an unlabeled independent bond $E$ between $a$ and $b$. We will assign a label to this edge to indicate the rigid cluster it belongs to. Currently, the cluster consists of only $E$.
3. Using the directed search from the edges connected to $a$ and $b$, we free $l$ pebbles and bring them to sites $a$ and $b$. These pebbles are now locked to $E$.
4. We loop over all sites $a'$ connected to $a$ and $b$ and see if we can free a pebble at $a'$ using the directed search.
5. If we can free a pebble at $a'$ then this site is floppy with respect to $E$ and so are all the sites visited during the search.
6. If we cannot free a pebble at $a'$ then this site is rigid with respect to $E$ and so are all the sites visited during the search. We assign the label of $E$ to all the edges connecting the rigid sites.
7. We remove all identification of rigid and floppy and consider the next unlabeled edge.

At the end of this process, all independent bonds are assigned a label indicating the rigid cluster it belongs to. Therefore the system has been decomposed into rigid clusters which are mutually floppy. We have also identified the over-constrained regions. The number of free pebbles at the end of the process indicates the number of degrees of freedom the system has or the number of floppy modes. Identification of percolating clusters is discussed in section IV.

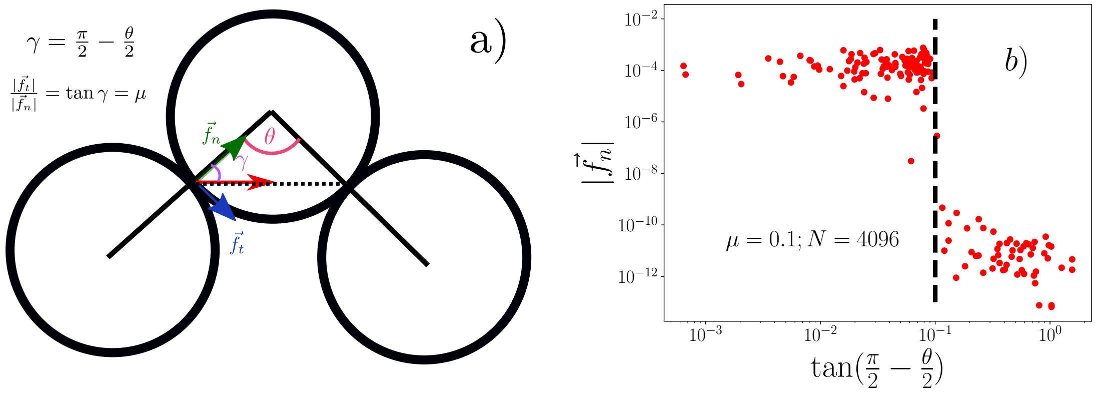


FIG. 1. **Minimum contact angle required for force-balance. a)** The schematic shows a particle with two contacts with an angle $\theta$ between the contacts. The red arrow, green and blue arrows depict the total, normal and tangential force at the contact respectively. For the central particle to be force-balance the total contact force (red arrow) should be along the dotted line depicted. Therefore the angle between the total contact force and the normal force should be $\gamma = \frac{\pi}{2} - \frac{\theta}{2}$. However, the maximum angle between the total contact force and the normal force is constrained by the Coulomb condition $\frac{|\vec{f}_t|}{|\vec{f}_n|} = \mu$. Therefore the minimum angle $\theta$ such that the central particle can be in force-balance with finite forces is such that $\mu < \tan(\frac{\pi}{2} - \frac{\theta}{2})$. **b)** Normal force magnitude (for a contact) as a function of the angle between contacts for particles with two contacts shown for a single configuration with $\mu = 0.1$. This shows that when $\mu < \tan(\frac{\pi}{2} - \frac{\theta}{2})$, there cannot be finite forces along the contacts.

## III. IDENTIFYING RATTLERS

Given configurations in force balance, we can remove rattlers. We recursively remove all particles with just one contact as those contacts cannot carry forces. In addition, we recursively remove all particles with two contacts such that the angle between the two contacts $\theta$ satisfies $\mu < \tan(\frac{\pi}{2} - \frac{\theta}{2})$. This is the minimum angle between two contacts such that the particle is in force-balance as shown in Fig. 1 with finite forces. $Z_{NR}$ is the average coordination number of the remaining system.

## IV. $P_\infty$ FOR FINITE RATE SHEAR WITH $\mu = 1.0$

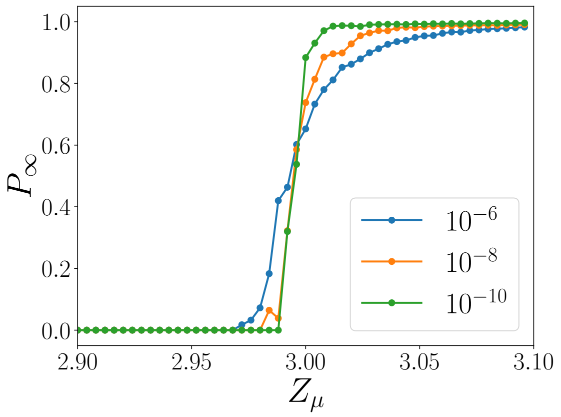


FIG. 2. $P_\infty$ **for three different shear rates.** The transition becomes sharper for lower shear rates.

We calculate $P_\infty$, the probability that a given disk belongs to a rigid cluster spanning in both $x$ and $y$ directions. For this analysis we consider the largest rigid cluster in the system and check if this cluster spans in both $x$ and $y$ direction. To do this, we consider the system along with 8 adjacent images. If the largest rigid cluster in the system does not span in either direction then when considered along with the images, the number of clusters (when one

considers only the largest cluster) in the system will be 9. If the largest cluster spans only in one direction, then when considered along with images, the number of clusters will be 3. In the case of the largest cluster spanning both directions, the number of cluster will be 1. For each strained sample we identify the rigid cluster which spans in both directions and compute $P_\infty = N_{largest}/N$. We bin $P_\infty$ based on $Z_\mu$ of the configuration and plot the average $P_\infty$ per bin. The result of this analysis is shown in Fig. 2. This shows that for finite shear rates, the transition is continuous although it gets sharper as one reduces the shear rate.

## V. RIGIDITY TRANSITION FOR SYSTEM WITH $\mu = 0.1$

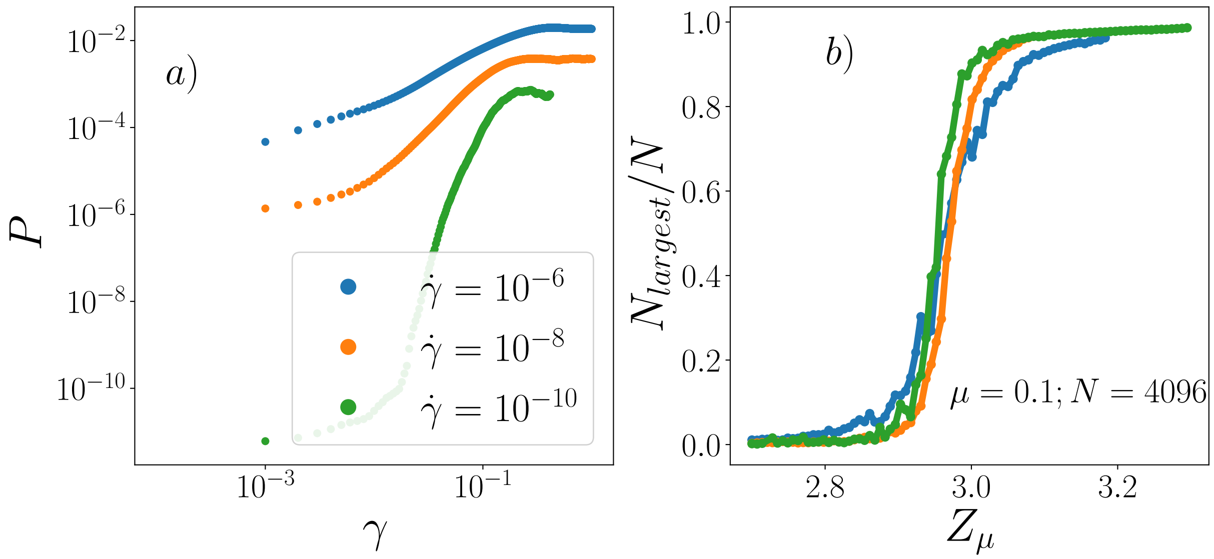


FIG. 3. **Results for** $\mu = 0.1$. **a)** Evolution of stress $\sigma_{xy}$ is similar to that of the high friction case described in the main text. **b)** The transition for $\mu = 0.1$ does get sharper as one lowers the shear rate. however, is less pronounced than how it is for $\mu = 1.0$. In addition, the transition seems to occur before the isostatic value $Z_\mu = 3.0$. The number of mobilized contacts $n_m$ is computed as number of contacts having $\frac{|\vec{f}_t|}{|\vec{f}_n|} > \mu - 10^{-8}$ per particle. As described in the main text, for the pebble game analysis we remove all particles with one contact.

### A. Finite rate shear

Finite rate shear simulations are performed at three different rates: $\dot{\gamma} = 10^{-6}, 10^{-8}, 10^{-10}$ for a system of $N = 4096$ particles. The behavior of the $\mu = 0.1$ system when $\dot{\gamma}$ is lowered is similar to what is observed for $\mu = 1.0$. Noticeably the transition occurs around $Z_\mu = Z_{NR} - n_m = 3.0$.

### B. Quasi-static shear with $\mu = 0.1$.

Here we discuss the associated results when shear simulations are performed quasi-statically for $\mu = 0.1$. We change the constant associated with global damping to a smaller number $\eta = 0.1$ as mentioned in Table. I. These give us better force-balanced configurations because simulations with a higher value of $\eta$ have significant viscous forces which contribute to the force balance of the particles. Using a lower $\eta$ reduces the effect of the viscous forces since we are interested in mechanical force balance. This contact network is analyzed using the pebble game algorithm with the results shown in Fig. 4. In this case as well, the transition is correctly identified by $Z_\mu$ crossing 3. Fig. 4 also shows that the rigidity transition occurs abruptly with the rigid percolating cluster. Here in addition to identifying mobilized contacts using the threshold $\delta$, we also consider contacts with $|\vec{f}_n| < 10^{-7}$ also to be sliding contacts as the tangential force is very small, in addition to the normal force. (See discussion on mobilized particles)

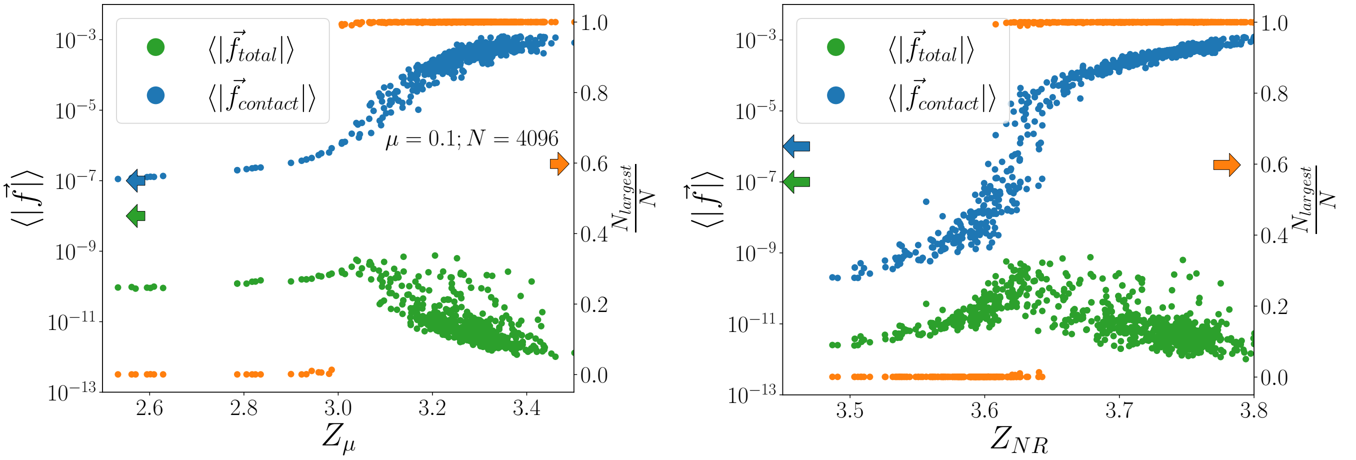


FIG. 4. **Result of pebble game analysis for $\mu = 0.1$. LEFT** These results show that for quasi-statically sheared systems the emergence of a rigid cluster in the system is instantaneous, as shown in the main text for $\mu = 1$. The number of mobilized contacts $n_m$ is computed as number of contacts having $\frac{|\vec{f}_t|}{|\vec{f}_n|} > \mu - 10^{-8}$ per particle as well as contacts with $|\vec{f}_n| < 10^{-7}$ (see discussion on mobilized contacts). **RIGHT** Same data shown with respect to $Z_{NR}$

## VI. DETERMINING MOBILIZED CONTACTS

Here we show how the threshold to identify mobilized contacts is calculated in different scenarios. As discussed in the main text, a contact is considered mobilized if $\frac{|\vec{f}_t|}{|\vec{f}_n|} > \mu - \delta$ where $\delta$ is the threshold. In this section, we show the effect of $\delta$ on our results. For the high friction case considered ($\mu = 1.0$), the number of mobilized contacts is low as shown in previous works [6–8]. Therefore the effect of the choice of the threshold is more pronounced for the $\mu = 0.1$ where the number of mobilized contacts is significant. Choice of $\delta$ affects the results of pebble game as the number of edges in the graph analyzed depends on $\delta$. Choosing a larger $\delta$ results in fewer edges in the graph as we replace each sliding contact with a single edge and others with a double edge. Therefore it is "easier" for the pebble game to detect a rigid cluster for smaller value of $\delta$ and otherwise.

We confine the discussion of identifying mobilized contacts to just the quasi-static case. In the case of quasi-static shear, we can unambiguously detect the shear jamming transition from the presence of the finite force contact network. The correct $\delta$ should therefore detect the rigid or over-constrained network at the strain value where finite forces exist. As we show this happens only at an intermediate value of $\delta$. A related point that needs to be discussed is how finite forces are identified given the limitations of the numerical procedure used. For unjammed configurations as well, DEM relaxation method does not completely remove the overlaps such that the forces are numerically zero. Instead as can be seen in Fig. 1 (b), one can categorize forces into finte and non-finite depending on the magnitude. Therefore we consider $|\vec{f}_{contact}| \geq 10^{-7}$ to be finite forces. For weak contact forces mobilization cannot be meaningfully computed.

We consider shear jamming of a single sample with $\mu = 0.1$ (Fig. 5 (a) and (b)) and $\mu = 1.0$ (Fig. 5 (c)). As shown in Fig. 5 (a), the transition to finite forces is correctly identified by $\delta = 10^{-3}, 10^{-6}$, while $\delta = 10^{-6}, 10^{-8}$ detects a rigidity transition at an earlier strain. We consider this first transition to be spurious and an artifact of inadequate numerical relaxation as the forces do no undergo a transition at this strain. The rigidity transition associated with the occurrence of finite forces in the system is discontinuous. To circumvent this issue we identify contact forces with $|\vec{f}_n| < 10^{-7}$ to be sliding contacts as these particles can be considered to be weakly in touch. We choose $\delta = 10^{-8}$ for analysis of configurations with $\mu = 0.1$ and $\delta = 10^{-12}$ for configurations with $\mu = 1.0$.

## VII. OVER-CONSTRAINED NETWORKS AND FLOPPY MODES IN FRICTIONAL AND FRICTIONLESS SHEAR

Here we highlight interesting differences of the rigidity transition in jamming from rigidity transition in other networks. For rigidity percolation studies in bond-diluted lattice systems, redundant bonds exist inside non-percolating rigid clusters alongside floppy modes in the system [4]. This is in contrast to jamming in frictionless and frictional disk packings, where redundant bonds do not appear in the system until the jamming transition where a percolating

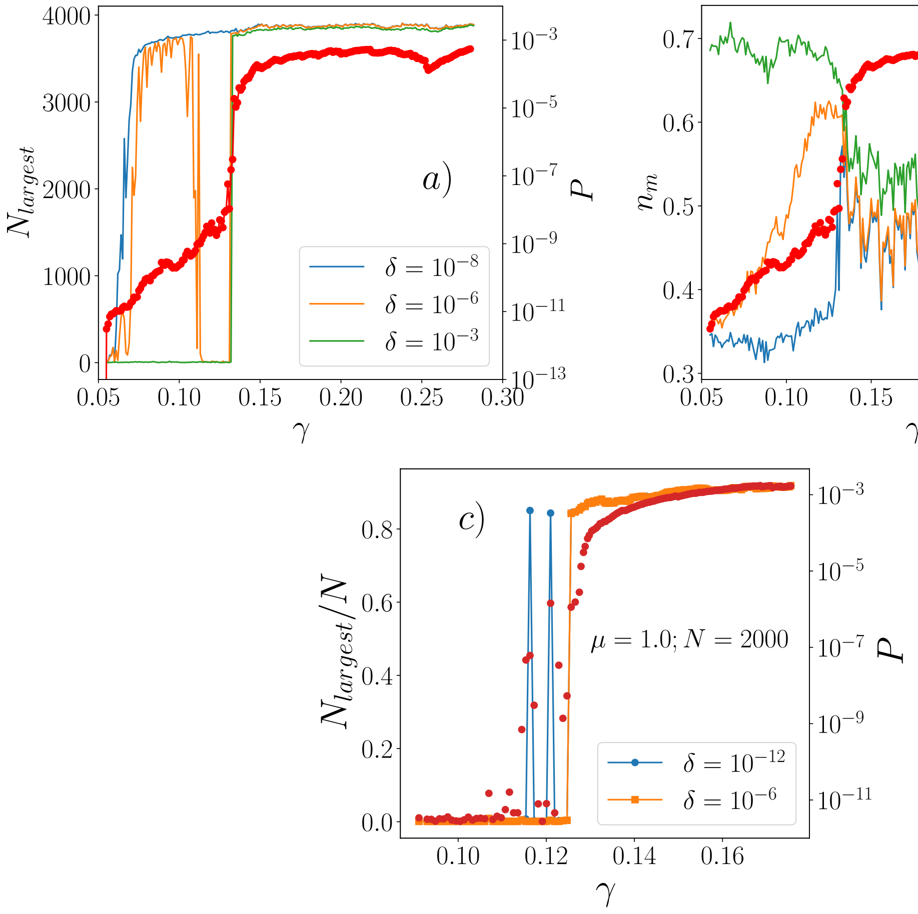


FIG. 5. **Rigidity transition associated with shear jamming for different $\delta$, where $\delta$ is the threshold for identifying mobilized contacts**. **a)** If we consider the presence of finite forces to be where shear jamming transition occurs with finite forces being defined as $P > 10^{-7}$, then $\delta = 10^{-3}, 10^{-6}$ detects a rigidity transition correctly. As explained in the text, $\delta = 10^{-8}$ detects a transition much earlier. We consider the rigidity transition detected by $\delta = 10^{-6}, 10^{-8}$ in the strain interval $[0.05, 0.1]$ to be spurious and an artifact of inadequate numerical relaxation. **b)** The fraction of mobilized contacts $n_m$ for the corresponding sample. The difference is the number of mobilized contacts is most pronounced before the jamming transition and a high value $n_m$ corresponds to floppy regions with no system spanning rigid cluster **a)** and **b)** Show a single sample with $\mu = 0.1$. **c)** Dependence of rigidity transition on the choice of $\delta$ for $\mu = 1.0$ quasi-static shear. Given that the number of mobilized contacts is very small for high friction, the choice of $\delta$ does not make a significant difference.

rigid cluster emerges which comprises of the whole system. In addition, floppy modes are not present in the system after jamming, provided that rattlers are removed. This is why Maxwell counting gives a very good identification of jamming transition since all bonds added are independent until jamming. These results are summarised in Fig. 6. We observe that the procedure followed in [9] does not capture this feature of jamming as shown in Fig. 6 (c) and (d).

---


[1] Stefan Luding. Cohesive, frictional powders: contact models for tension. *Granular matter*, 10(4):235–246, 2008.
[2] Steve Plimpton. Fast parallel algorithms for short-range molecular dynamics. *Journal of computational physics*, 117(1):1–19, 1995.
[3] Gerard Laman. On graphs and rigidity of plane skeletal structures. *Journal of Engineering mathematics*, 4(4):331–340, 1970.
[4] Donald J Jacobs and Bruce Hendrickson. An algorithm for two-dimensional rigidity percolation: the pebble game. *Journal of Computational Physics*, 137(2):346–365, 1997.
[5] Audrey Lee and Ileana Streinu. Pebble game algorithms and sparse graphs. *Discrete Mathematics*, 308(8):1425–1437, 2008.

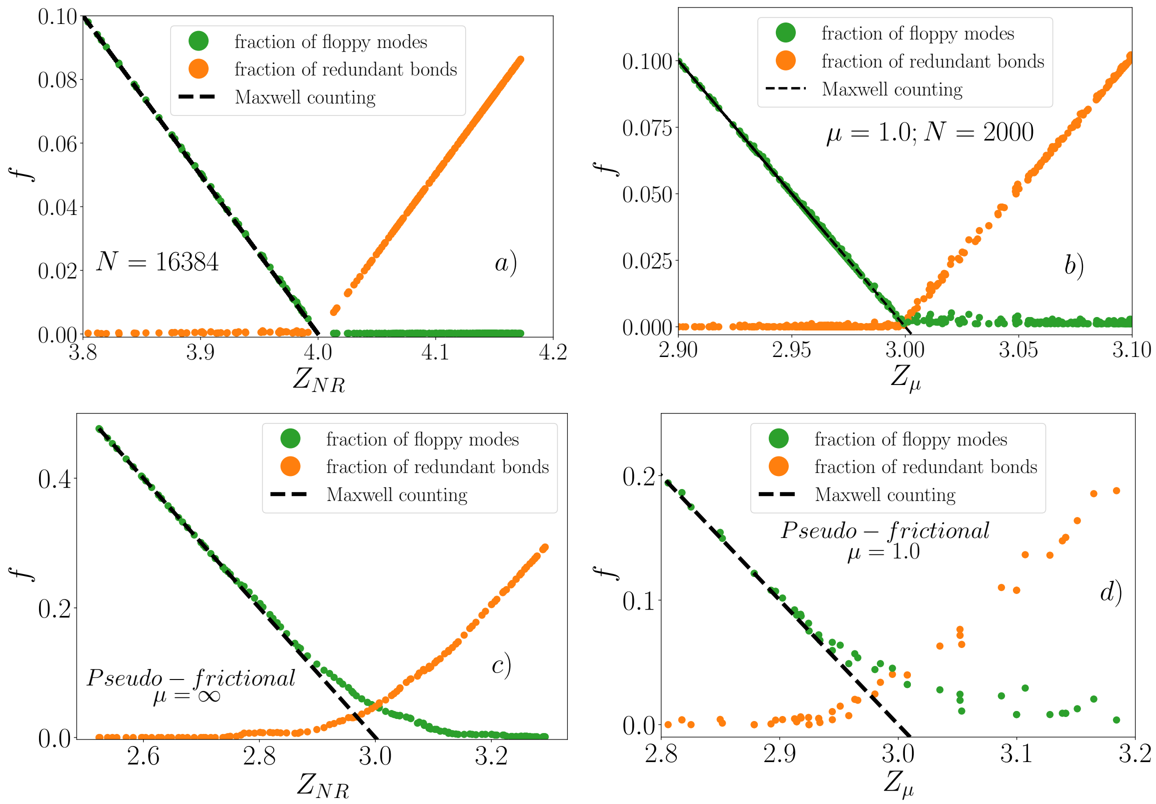


FIG. 6. **Fraction of redundant contacts and floppy modes in frictionless and frictional systems under shear. a)** Frictionless systems. **b)** Frictional system with $\mu = 1.0$. For both systems, redundant bonds do not appear until the jamming transition. Also once rattlers are removed, there are no floppy modes after jamming. Due to these reasons, Maxwell's counting correctly identifies the jamming and the rigidity transition. **c)** Redundant bonds and floppy modes in pseudo-frictional case analyzed in [9]. **d)** Pseudo-frictional case with finite friction coefficient $\mu = 1.0$


[6] Silke Henkes, Martin van Hecke, and Wim van Saarloos. Critical jamming of frictional grains in the generalized isostaticity picture. *EPL (Europhysics Letters)*, 90(1):14003, 2010.

[7] Silke Henkes, David A Quint, Yaouen Fily, and Jennifer M Schwarz. Rigid cluster decomposition reveals criticality in frictional jamming. *Physical review letters*, 116(2):028301, 2016.

[8] Kostya Shundyak, Martin van Hecke, and Wim van Saarloos. Force mobilization and generalized isostaticity in jammed packings of frictional grains. *Physical Review E*, 75(1):010301, 2007.

[9] HA Vinutha and Srikanth Sastry. Force networks and jamming in shear-deformed sphere packings. *Physical Review E*, 99(1):012123, 2019.
